# Supplementary material for: A Financial Brain Scan of the LLM
Source: arXiv:2508.21285 source file (2026-11-04)
Supplement: Supplementary file 1 [file 09_appendix.tex]

\clearpage
\appendix
